# Supplementary material for: Percolation thresholds on triangular lattice for neighbourhoods containing sites up-to the fifth coordination zone
Source: arXiv:2102.10066 source file (2021-04-13)
Supplement: Supplementary file 1 [file SupMat.pdf]

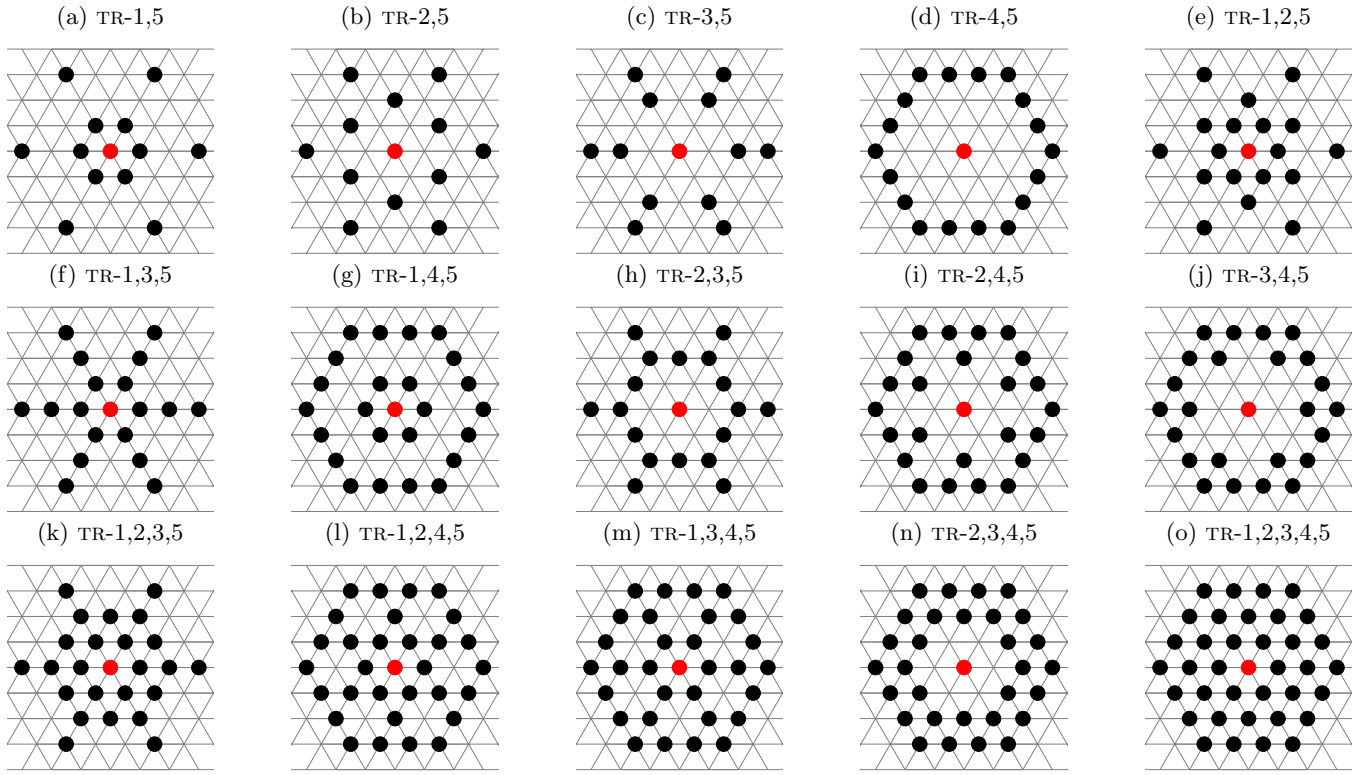

FIG. A1: Examples of neighborhoods containing the next-next-next-nearest neighbors on triangular lattice.

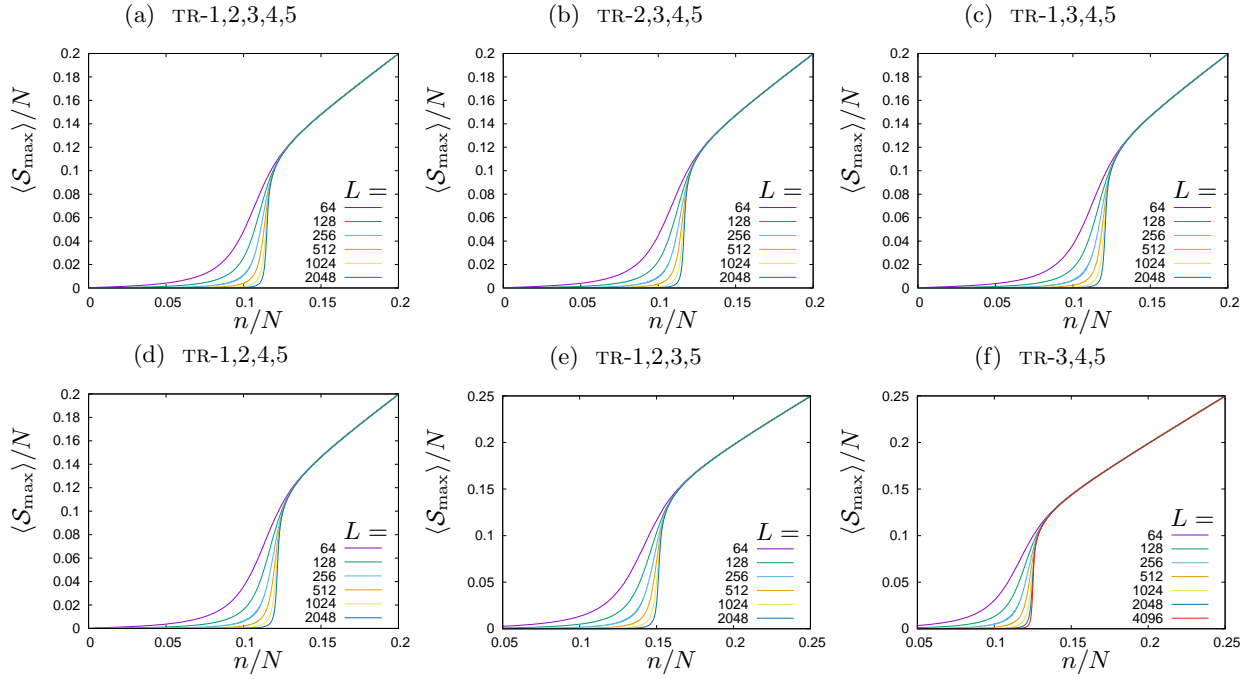

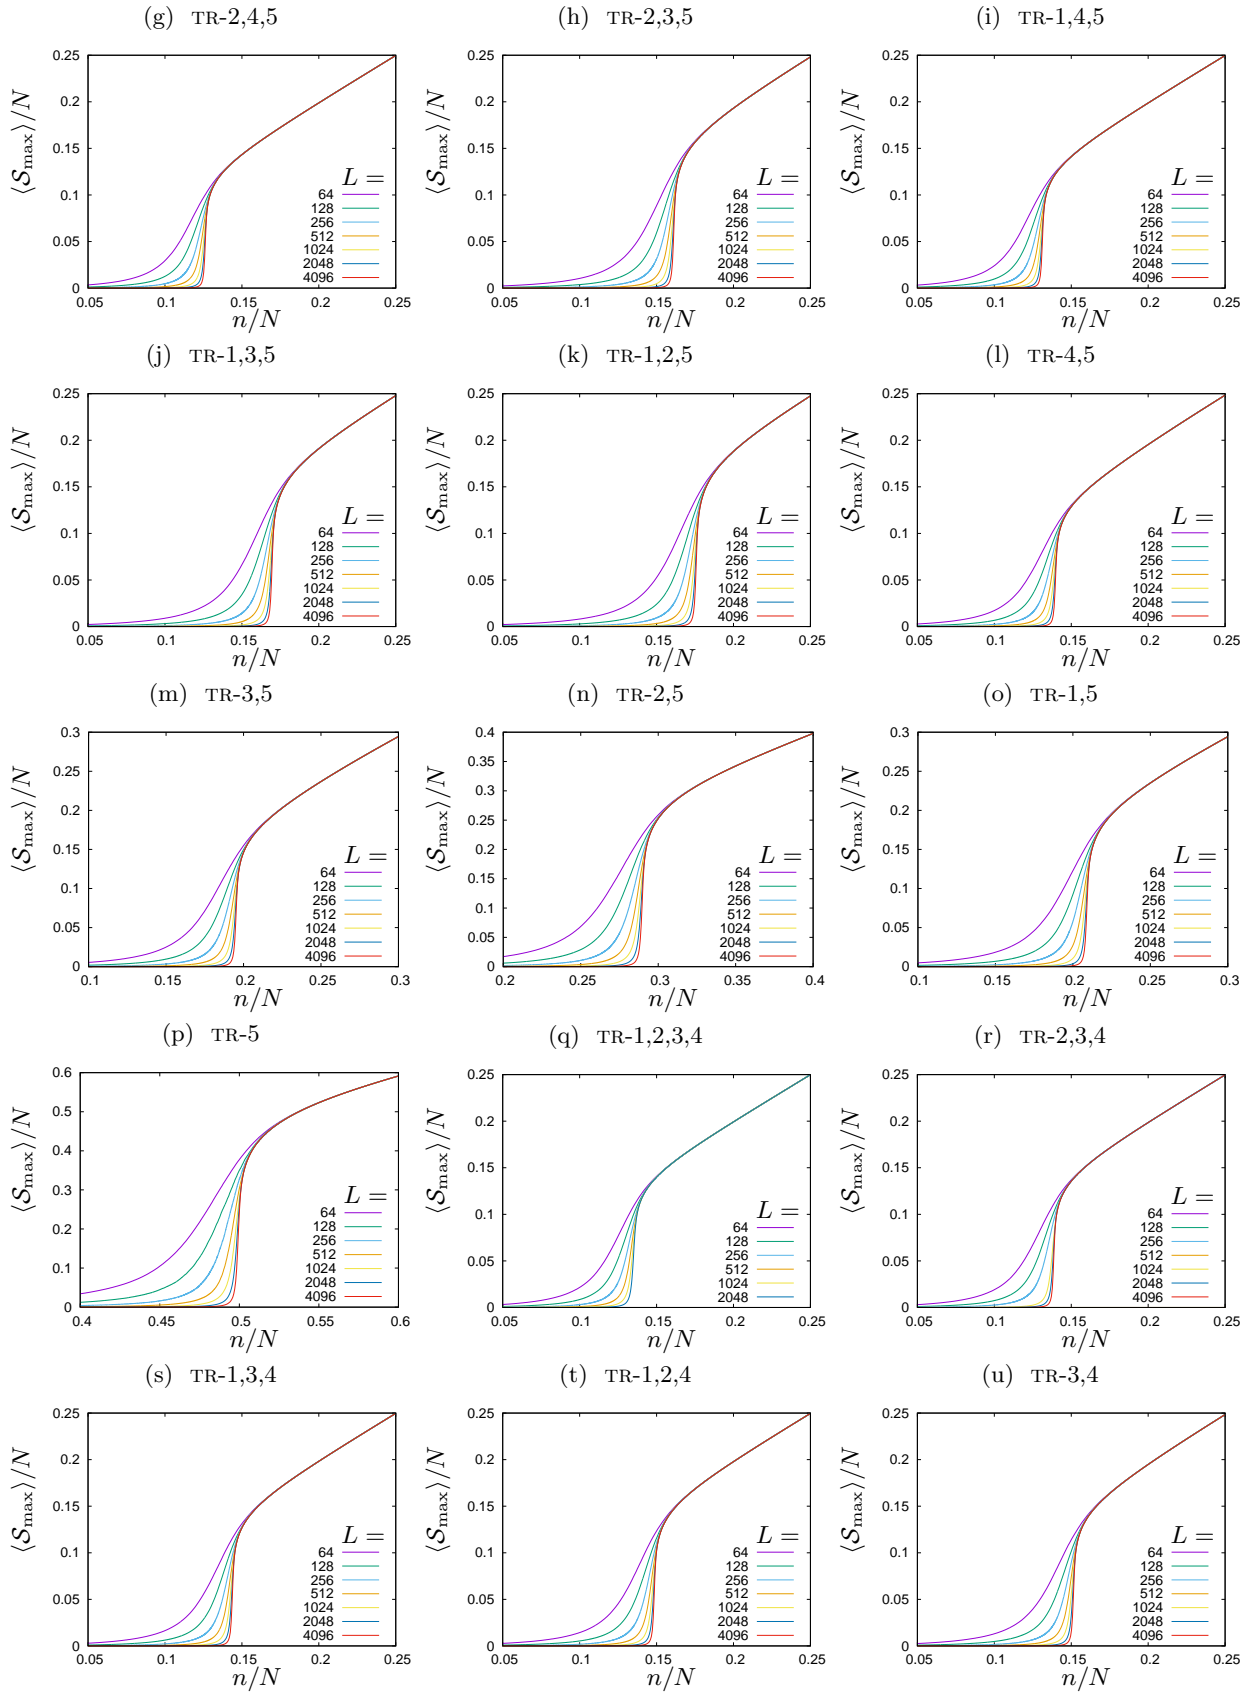

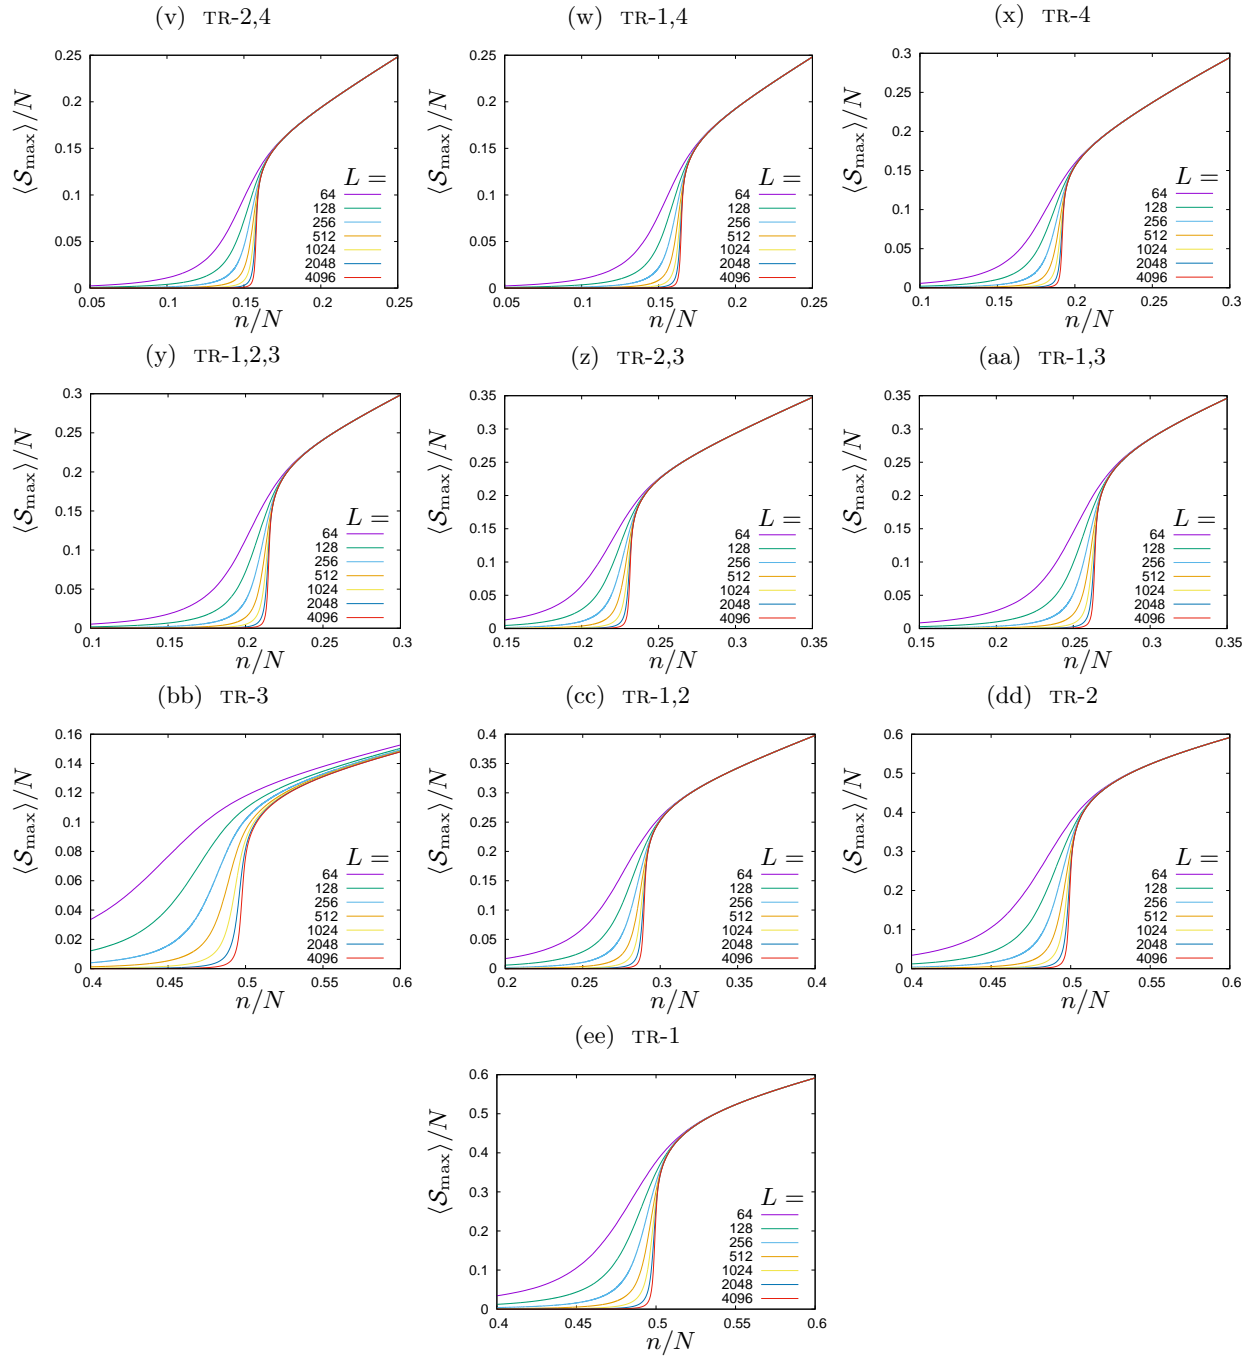

FIG. A2: Average the largest cluster size  $\langle S_{\max} \rangle$  vs. number of occupied sites, both normalized to the system size  $N$

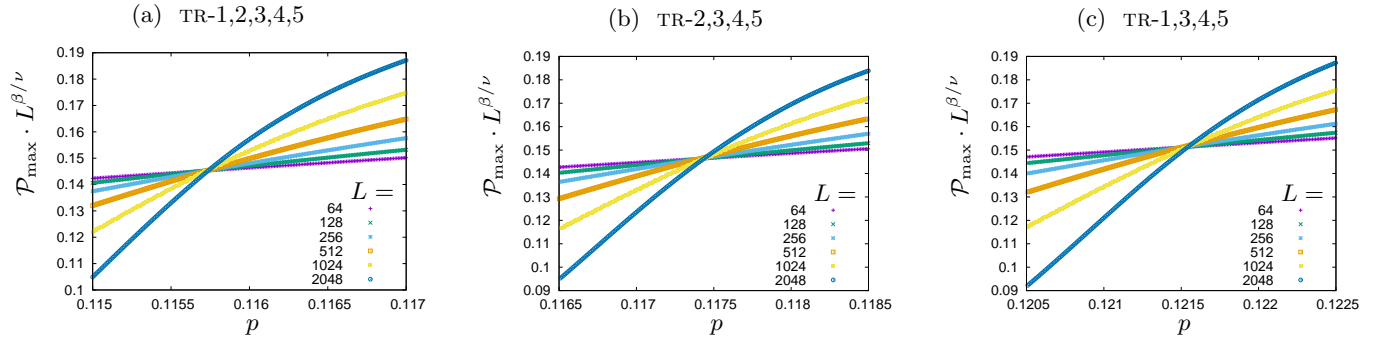

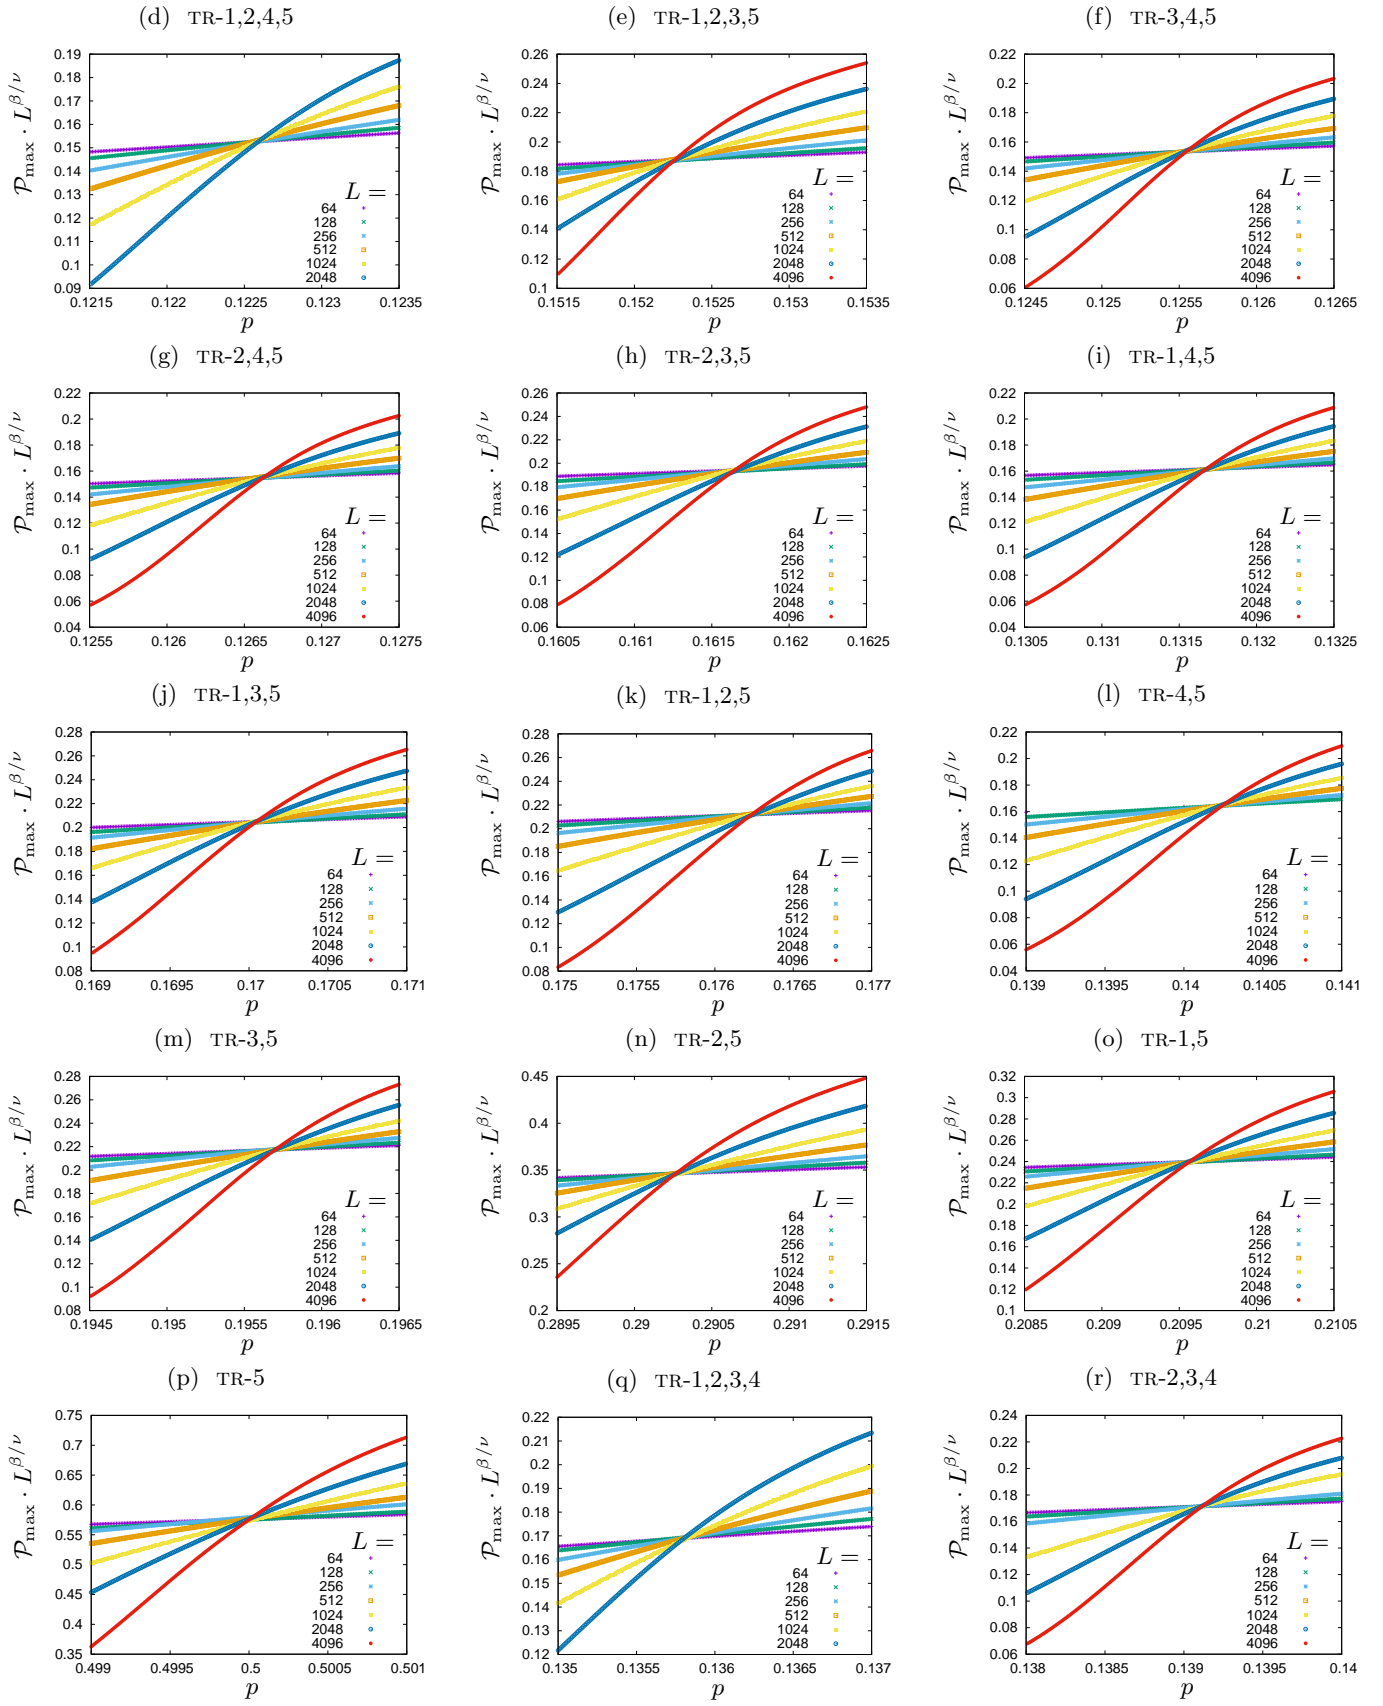

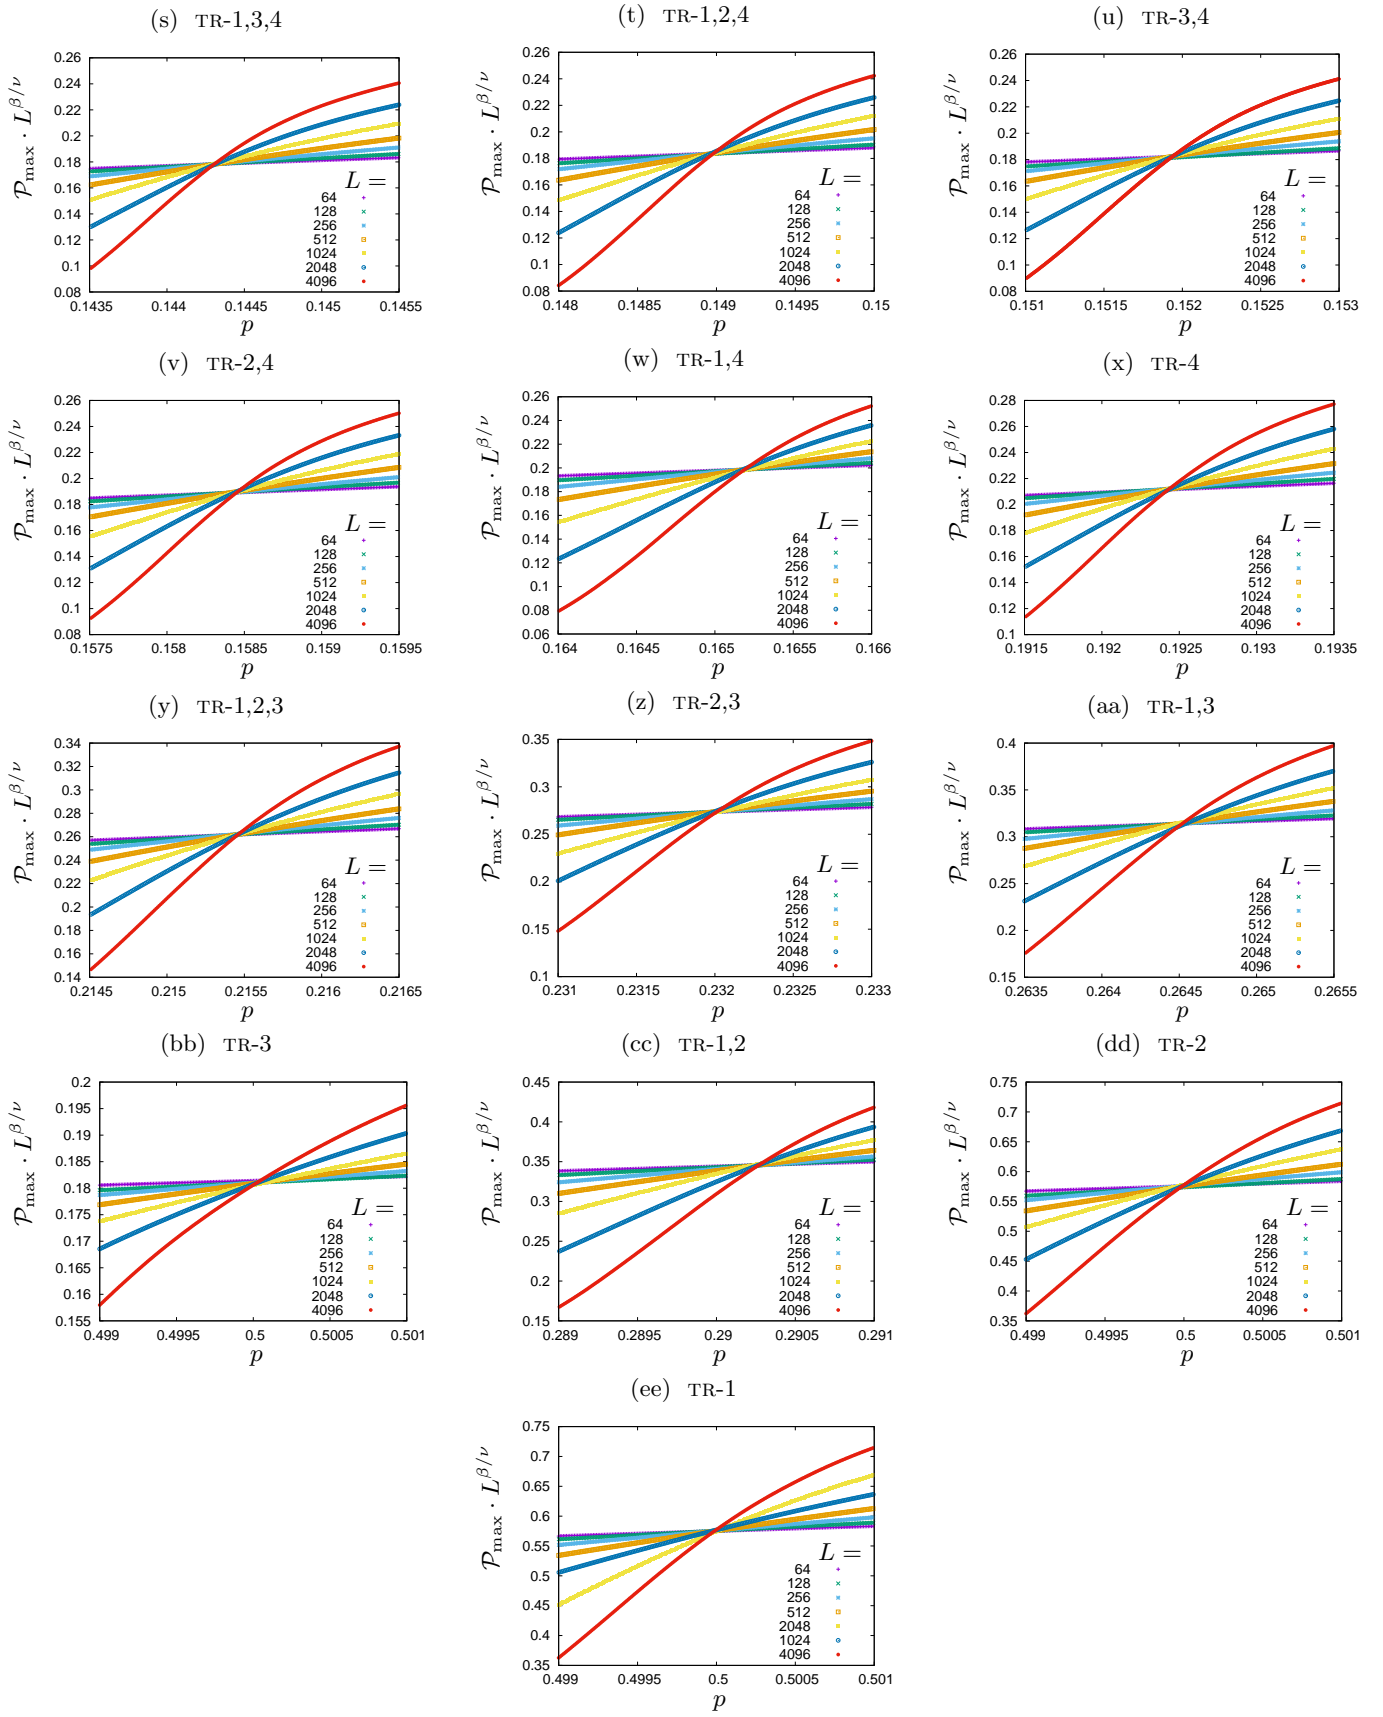

FIG. A3: Probability of belonging to the largest cluster  $\langle \mathcal{P}_{\max} \rangle$  vs. occupation probability  $p$

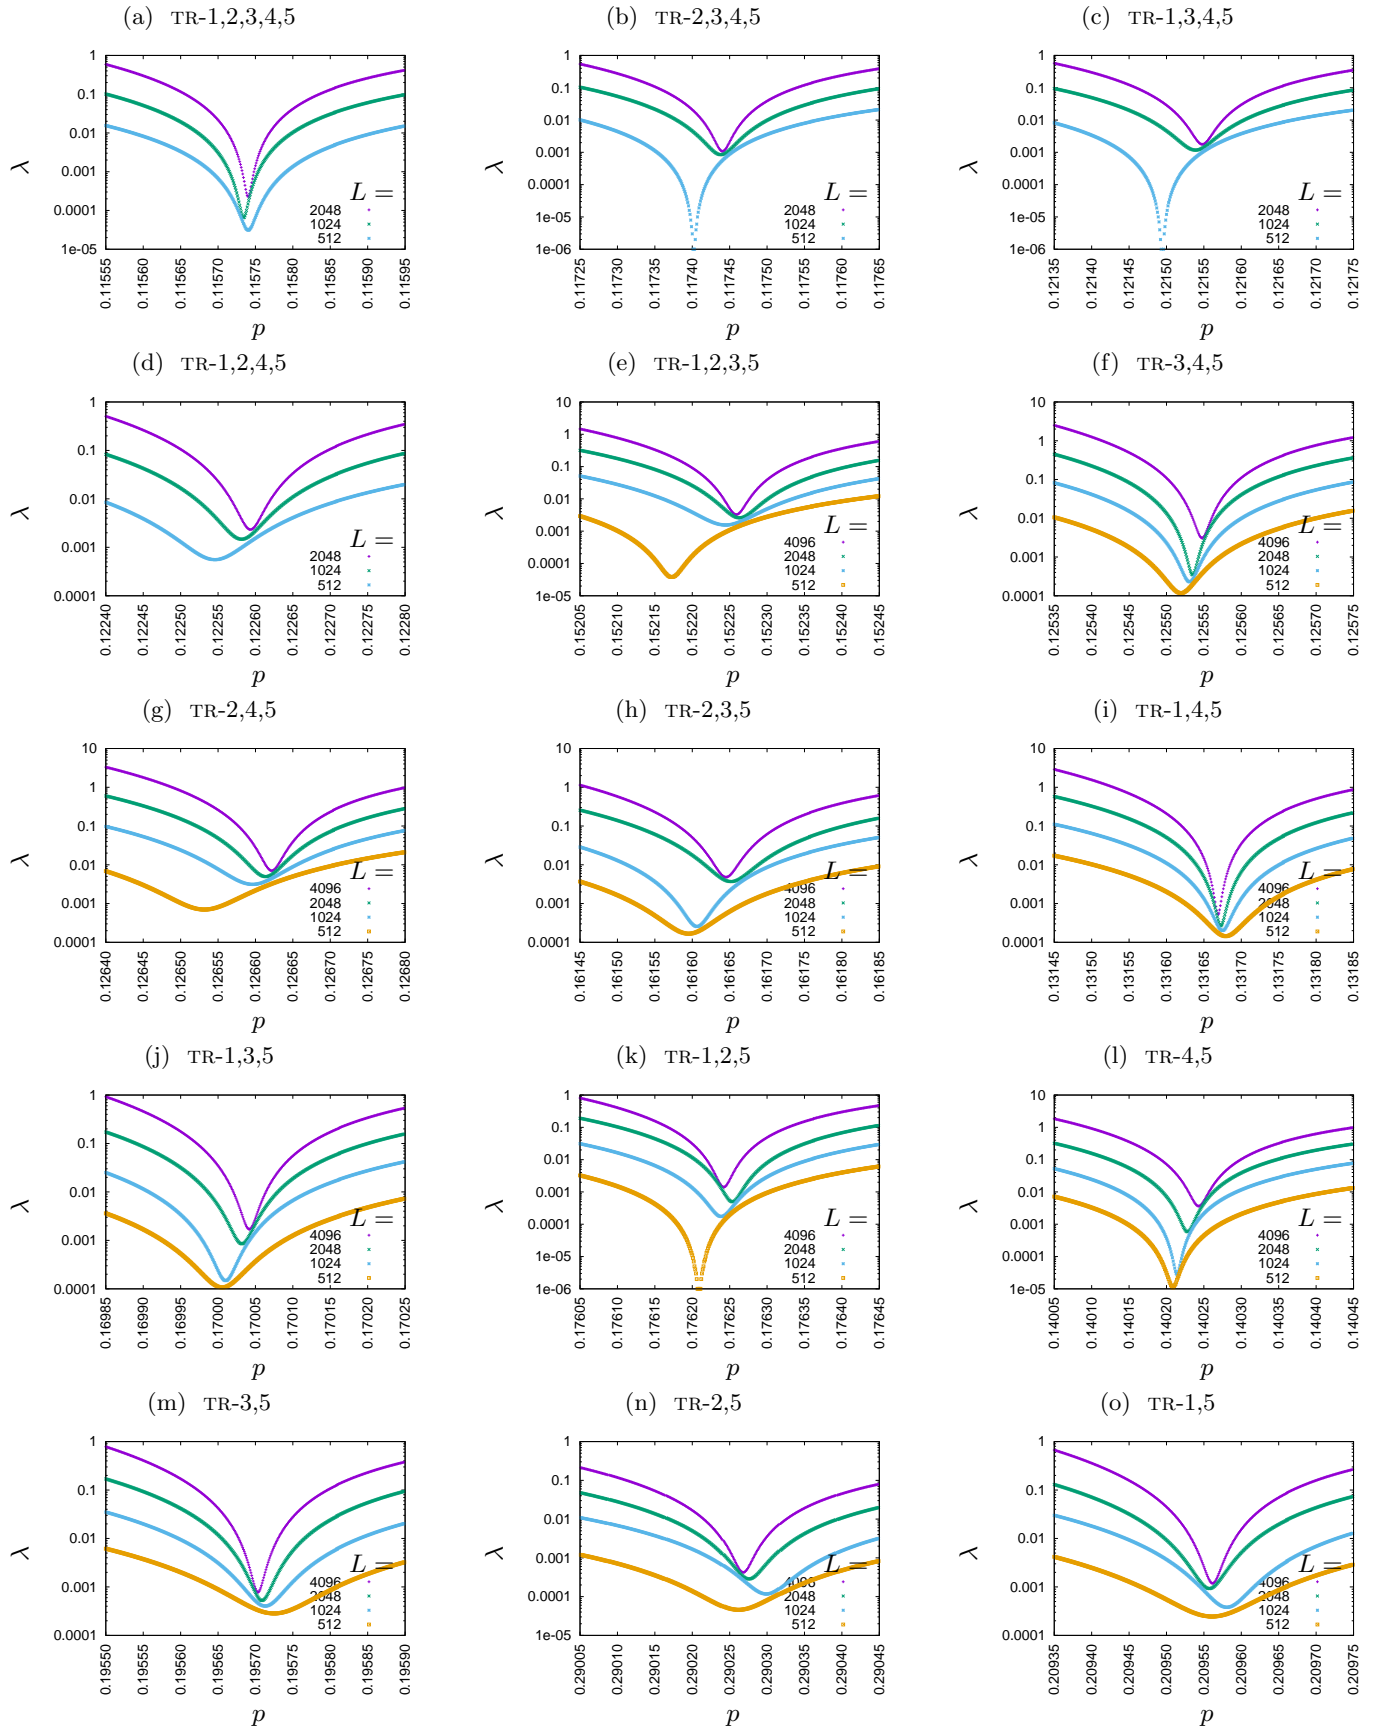

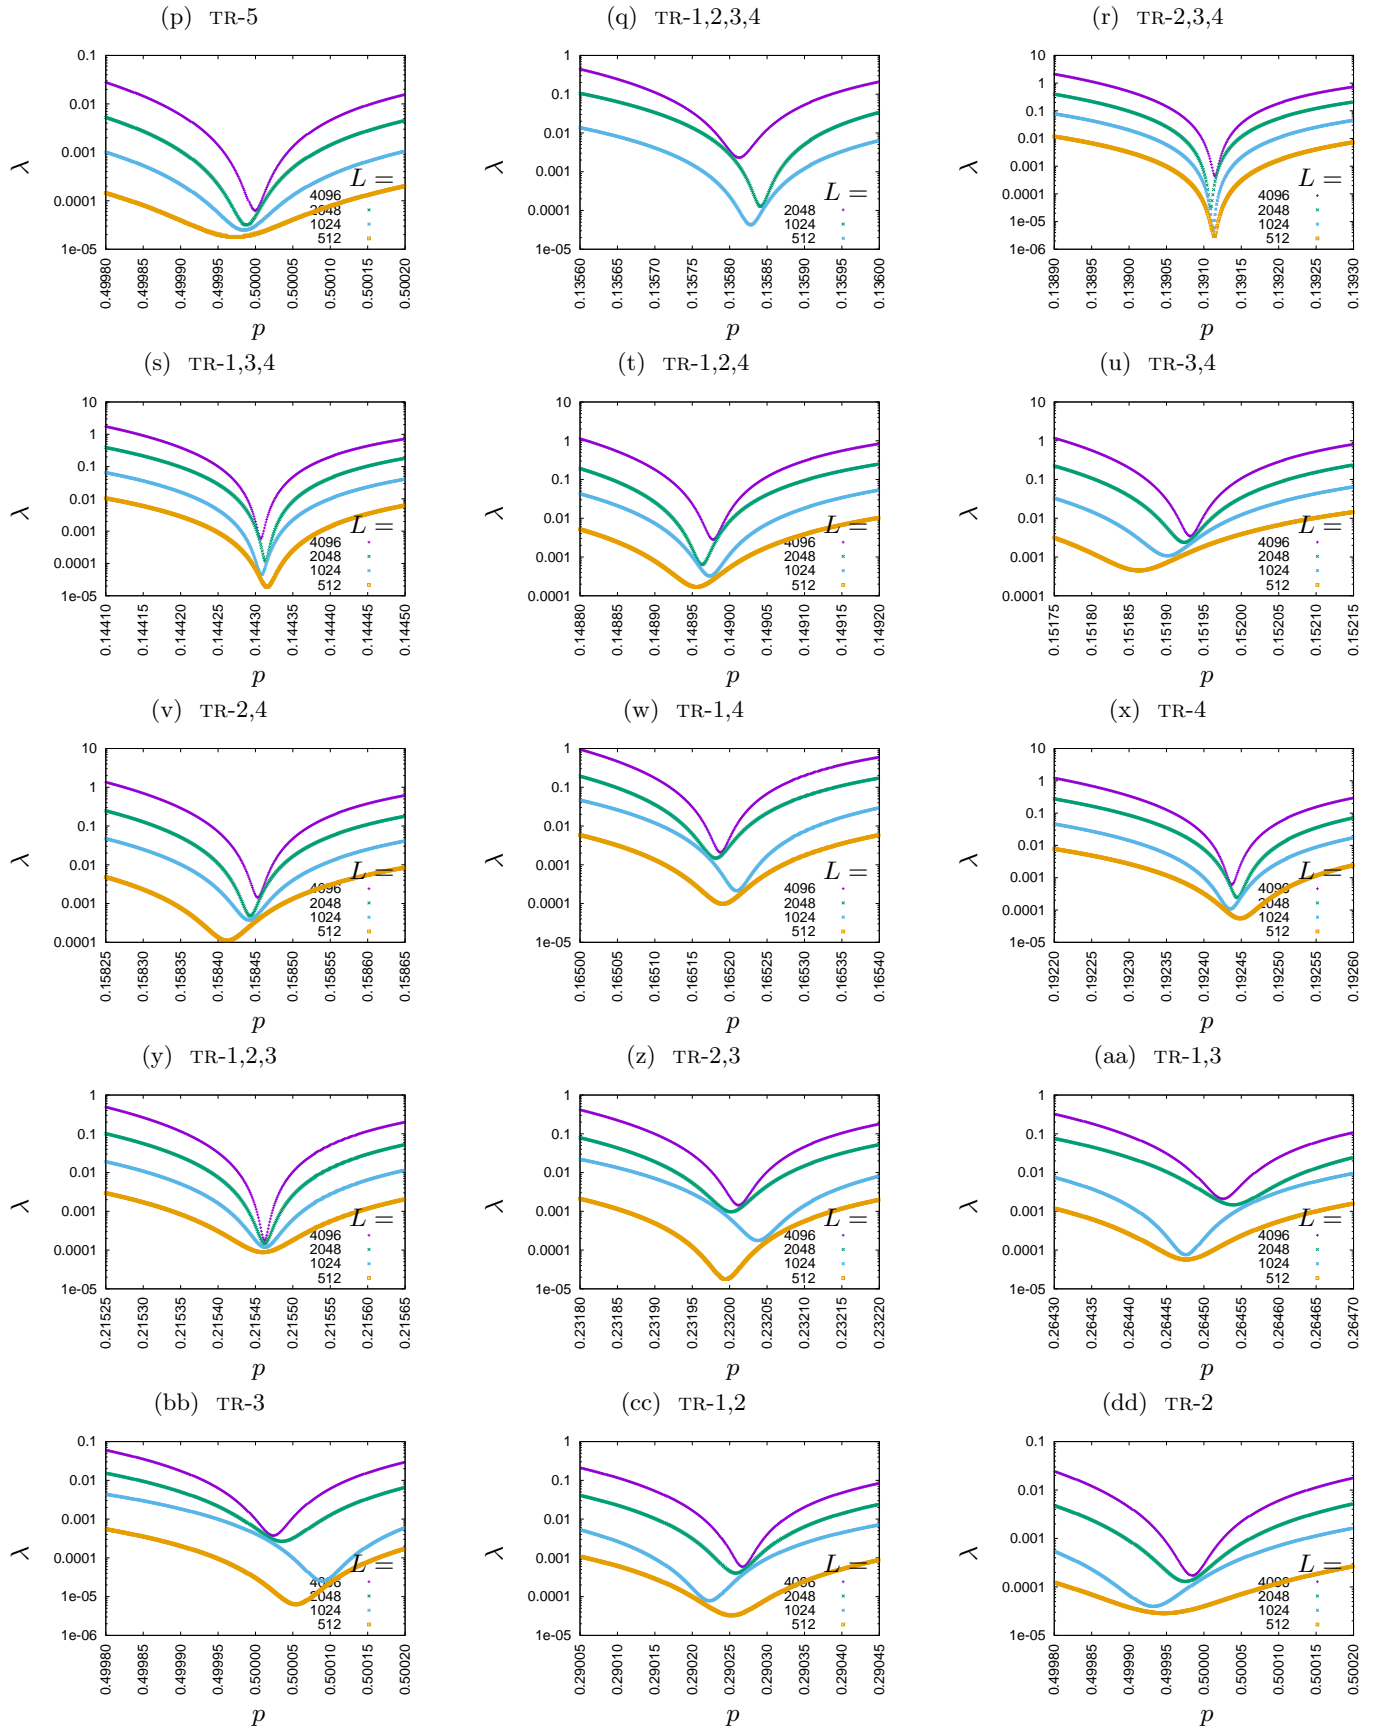

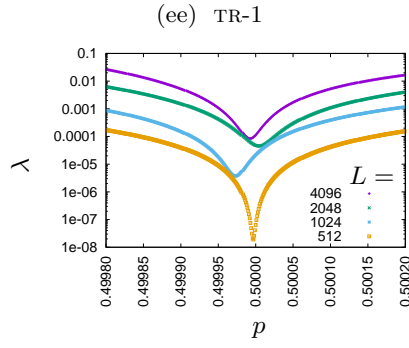

FIG. A4: Sum of pairwise differences  $\langle \lambda \rangle$  vs. occupation probability  $p$

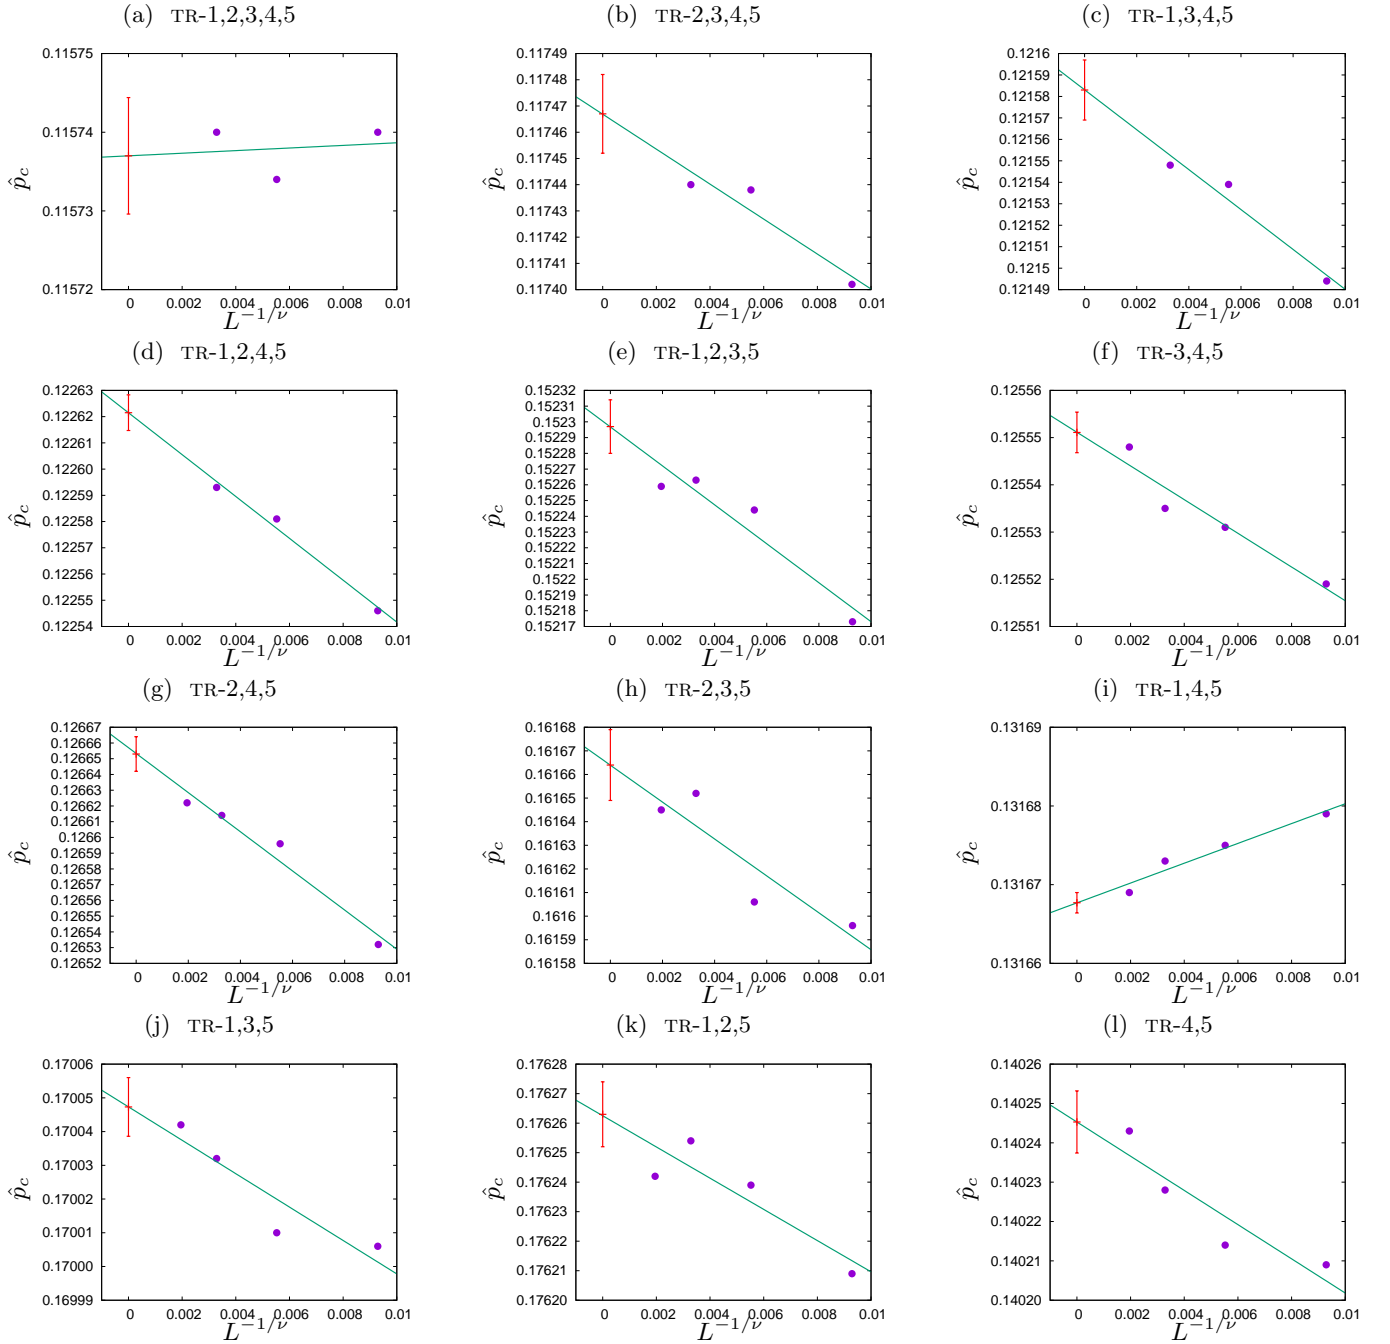



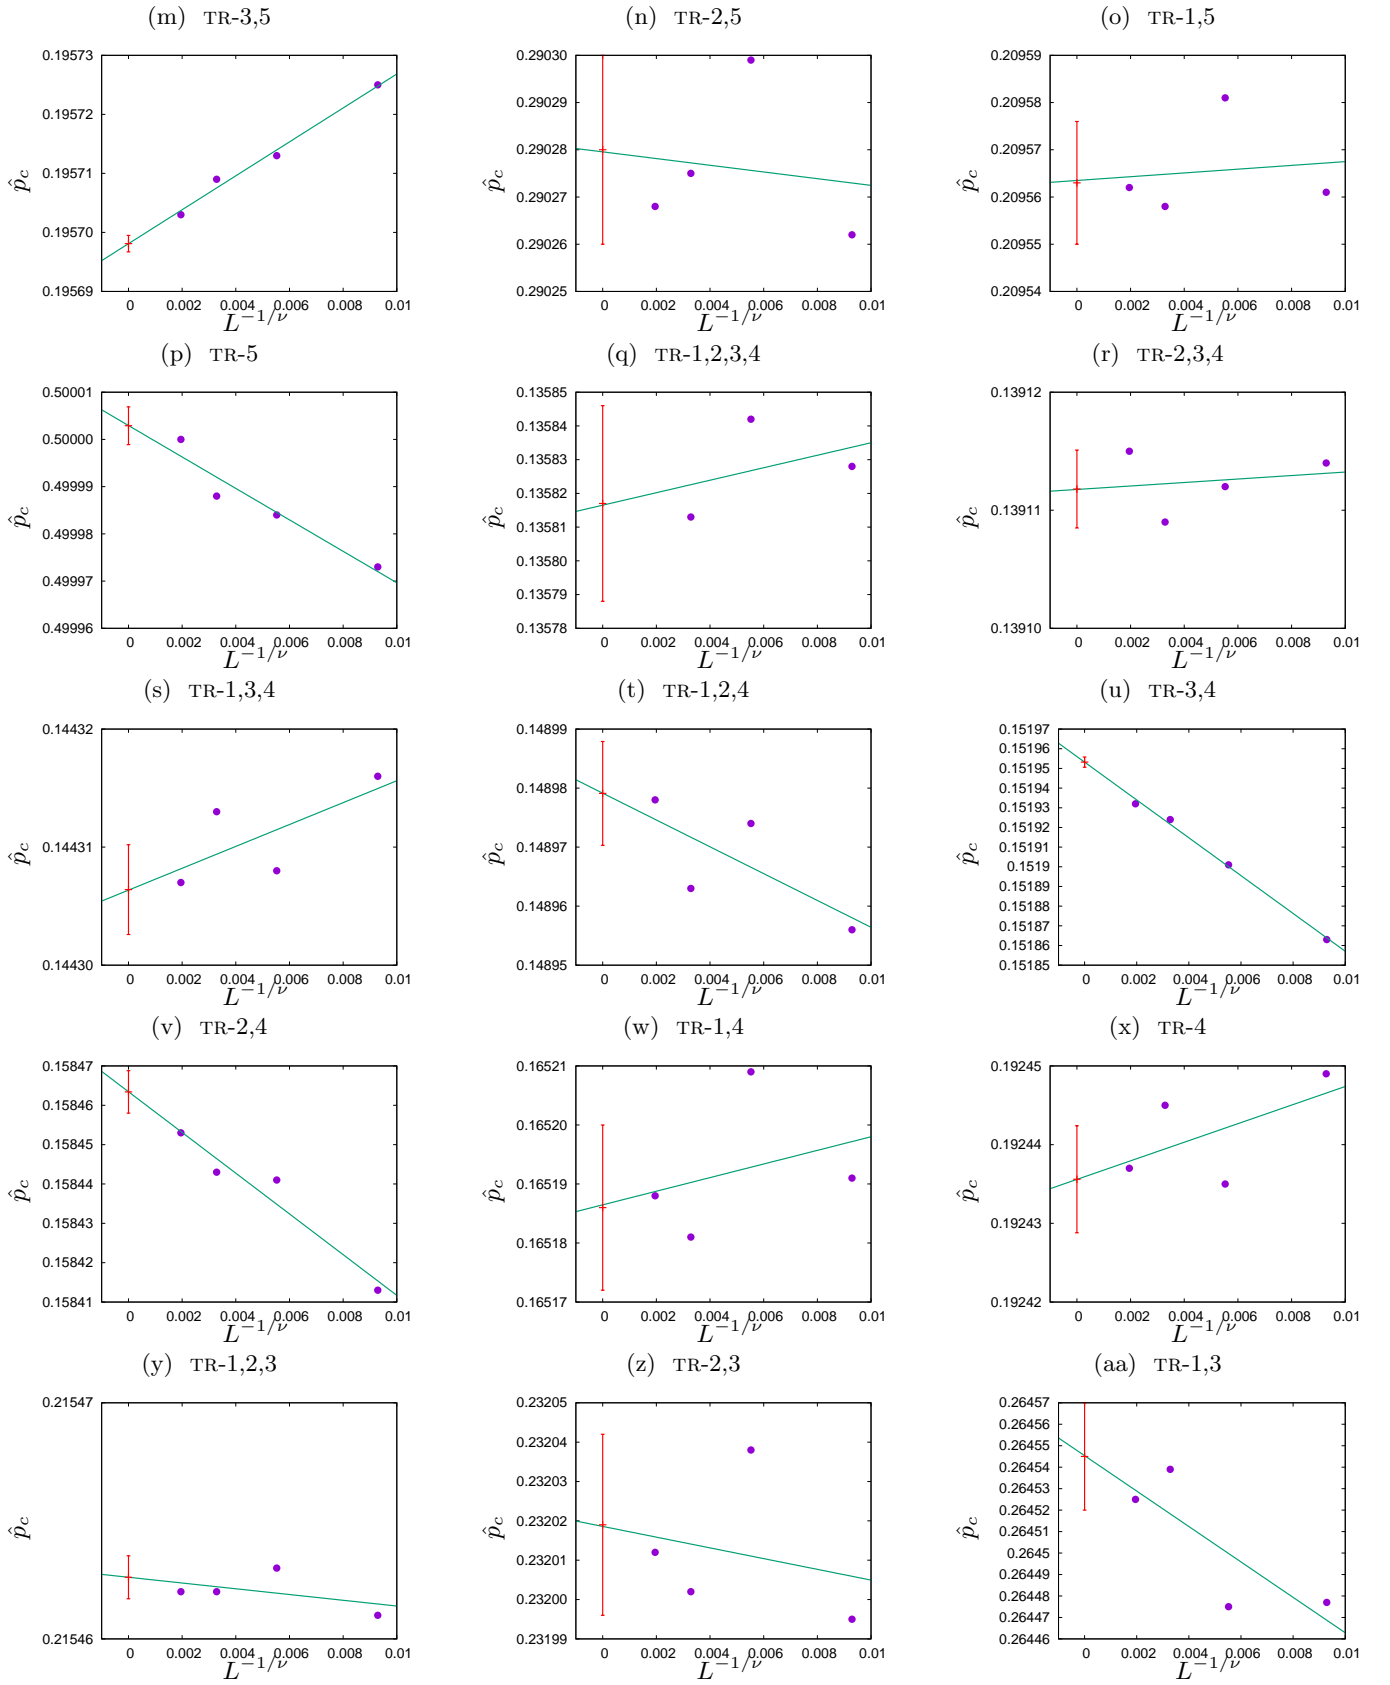

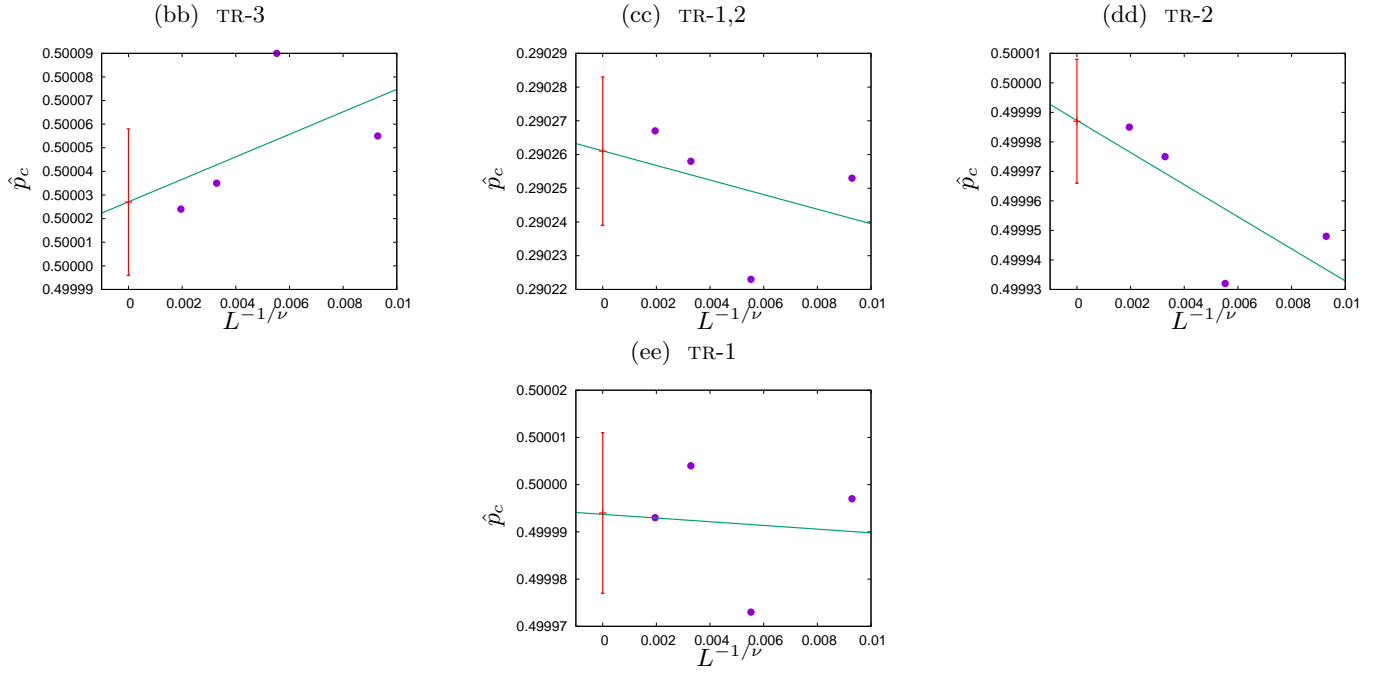FIG. A5: Finite size effect corrections to  $p_c$ .
